# Supplementary material for: How Much and When Do We Need Higher-order Information in Hypergraphs? A Case Study on Hyperedge Prediction
Source: arXiv:2001.11181 source file (2020-05-13)
Supplement: Supplementary file 1 [file appendix.tex]

\newpage
\section{Appendices}

If your work needs an appendix, add it before the
``\verb|\end{document}|'' command at the conclusion of your source
document.

Start the appendix with the ``\verb|appendix|'' command:
\begin{verbatim}
  \appendix
\end{verbatim}
and note that in the appendix, sections are lettered, not
numbered. This document has two appendices, demonstrating the section
and subsection identification method.

% List of things to write

% Full dataset statistics
% Dataset statistics
\begin{table*}[h]
  \small\addtolength{\tabcolsep}{5pt}
  \resizebox{\textwidth}{!}{
  \begin{tabular}{lcccccccccc}%{l|cccc|cc|cc|cc}
    \toprule
    \multirow{2}{*}{Dataset}
    & \multicolumn{4}{c}{\bf Hypergraph}
    & \multicolumn{2}{c}{\bf 2-projected graph}
    & \multicolumn{2}{c}{\bf 3-projected graph}
    & \multicolumn{2}{c}{\bf 4-projected graph}\\ 
    \cmidrule(lr){2-5}
    \cmidrule(lr){6-7}
    \cmidrule(lr){8-9}
    \cmidrule(lr){10-11}
    & \# unique hyperedges  
    & \# size 4 
    & \# size 5 
    & \# size 10 
    & \# nodes & \# edges
    & \# nodes & \# edges 
    & \# nodes & \# edges  \\
    \midrule
    email-Enron & 1,491 & 136 & 63 & 0
    & 143 & 1,442 & 1,210 & 21,885 & 2,871 & 123,638\\
    email-Eu & 24,223 & 2,294 & 1,359 & 0 \\
    contact-primary-school & 12,704 & 347 & 9 & 0 \\
    contact-high-school & 7,818 & 222 & 7 & 0\\
    NDC-classes & \\
    NDC-substances & \\
    DAWN & \\
    congress-bills & \\
    tags-ask-ubuntu & \\
    tags-math-sx & \\
    threads-ask-ubuntu & \\
    threads-math-sx & \\
    coauth-MAG-History & \\
    coauth-MAG-Geology & \\
    coauth-DBLP & 2,454,734 & 419,434 & 205,970 & 0
    & 443,845 & 723,382 & 569,179 & 4,214,637 & 654,471 & 16,945,418\\
  \bottomrule
  \end{tabular}}
  \ourcaption{Dataset statistics \kijung{Can we simplify this table? Some information might not be necessary.}\\} 
  \label{tab:datasets_full}
\end{table*}
% 1. Note that they are the number of "removed" hyperedges. 2. Nodes and vertices interchangeably. 3. Further statistics in appendix (dropbox link) 4. <=10

% Full experiment results

\begin{table*}[h]
  \small\addtolength{\tabcolsep}{5pt}
  \resizebox{\textwidth}{!}{
  \begin{tabular}{lcccccccccccc}
    \toprule
    \multirow{2}{*}{Dataset}
    & \multicolumn{6}{c}{\bf Only 2}
    & \multicolumn{6}{c}{\bf 2 to 3 utility (\%)}\\ 
    \cmidrule(lr){2-7}
    \cmidrule(lr){8-13}
    & GM & HM & AM & CN & JC & AA
    & GM & HM & AM & CN & JC & AA
    \\
    \cmidrule(lr){1-1}
    \cmidrule(lr){2-7}
    \cmidrule(lr){8-13}
    email-Enron & 14.91 & 1.36 & 63 & 0
    & 143 & 14.42 & -12.10 & 28.85 & 218.85 & 28.71 & 123.38 & 1234.38\\
    email-Eu & \\
    contact-primary-school & \\
    contact-high-school & \\
    NDC-classes & \\
    NDC-substances & \\
    DAWN & \\
    congress-bills & \\
    tags-ask-ubuntu & \\
    tags-math-sx & \\
    threads-ask-ubuntu & \\
    threads-math-sx & \\
    coauth-MAG-History & \\
    coauth-MAG-Geology & \\
    coauth-DBLP & \\
    \cmidrule(lr){1-1}
    \cmidrule(lr){2-7}
    \cmidrule(lr){8-13}
    Averaged & 100\\
  \bottomrule
  \end{tabular}}
\ourcaption{Performance\\}
\label{tab:performance_size4}
\end{table*}

\begin{table*}[h]
  \small\addtolength{\tabcolsep}{5pt}
  \resizebox{\textwidth}{!}{
  \begin{tabular}{lcccccccccccccccccc}
    \toprule
    \multirow{2}{*}{Dataset}
    & \multicolumn{6}{c}{\bf Only 2}
    & \multicolumn{6}{c}{\bf 2 to 3 utility (\%)}
    & \multicolumn{6}{c}{\bf 3 to 4 utility (\%)}\\
    \cmidrule(lr){2-7}
    \cmidrule(lr){8-13}
    \cmidrule(lr){14-19}
    & GM & HM & AM & CN & JC & AA
    & GM & HM & AM & CN & JC & AA
    & GM & HM & AM & CN & JC & AA\\
    \cmidrule(lr){1-1}
    \cmidrule(lr){2-7}
    \cmidrule(lr){8-13}
    \cmidrule(lr){14-19}
    email-Enron & 14.91 & 1.36 & 63 & 0
    & 143 & 14.42 & -12.10 & 28.85 & 218.85 & 28.71 & 123.38 & 1234.38\\
    email-Eu & \\
    contact-primary-school & \\
    contact-high-school & \\
    NDC-classes & \\
    NDC-substances & \\all
    DAWN & \\
    congress-bills & \\
    tags-ask-ubuntu & \\
    tags-math-sx & \\
    threads-ask-ubuntu & \\
    threads-math-sx & \\
    coauth-MAG-History & \\
    coauth-MAG-Geology & \\
    coauth-DBLP & \\
    \cmidrule(lr){1-1}
    \cmidrule(lr){2-7}
    \cmidrule(lr){8-13}
    \cmidrule(lr){14-19}
    Averaged & 100\\
  \bottomrule
  \end{tabular}}
\ourcaption{Performance  \kijung{Can we merge Tables 2 and 3? Is it okay to report only utilities?}\\}
\label{tab:performance_size5}
\end{table*}

% Stars and cliques

\begin{figure}[h]
\centering
\begin{subfigure}[c]{0.42\linewidth}
  \centering
  \includegraphics[width=\linewidth]{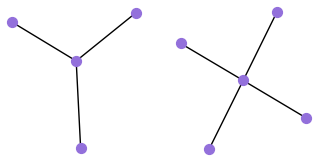}
  \ourcaption{Stars}
  \label{fig:ss} 
\end{subfigure}\hspace{0.12\linewidth}%
\begin{subfigure}[c]{0.42\linewidth}
  \centering
  \includegraphics[width=\linewidth]{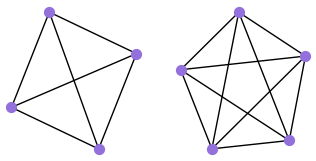}
  \ourcaption{Cliques}
  \label{fig:cc}
\end{subfigure}
\ourcaption{Two types of negative hyperedges generated from the pairwise projected graph. Higher-order utility is higher when discriminating cliques, which is more challenging.}
\label{fig:sscc}
\end{figure}
